# Supplementary material for: Recurrent neural networks approximate continuous functions
Source: arXiv:2606.20325 source file (2026-06-18)
Supplement: Supplementary file 11 [file tmnu-subroutines-appendix.tex]

\documentclass[../../main.tex]{subfiles}

\usepackage{xr-hyper}

\makeatletter
\@ifclassloaded{subfiles}{%
    \externaldocument{tmnu-model} % adjust path if needed
    \externaldocument{tmnu-construction-appendix} % adjust path if needed
}{}
\makeatother

\begin{document}

\end{document}
